# Supplementary material for: Multiscale Modelling of Lytic Polysaccharide Monooxygenases
Source: arXiv:1612.05513 source file (2017-02-07)
Supplement: Supplementary file 1 [file paper_SI_v1.pdf]

# Supporting information for: Multiscale Modelling of Lytic Polysaccharide Monooxygenases

Erik D. Hedegård* and Ulf Ryde*

*Department of Chemistry, Lund University, Kemicentrum Sölvegatan 39, Lund, Sweden*

E-mail: erik.hedegard@teokem.lu.se; ulf.ryde@teokem.lu.se

## 1 Coordinates for optimised structures

Coordinates for structures of **1**, **2** and **3** (all with protein "free") are given below.

```
   62
Cu rest state (1) TPSS-D3/def2-SV(P); Energy=-3169.58248468946
N 1.8469642 -12.3296119 -2.7479741
H 1.4433474 -11.5072242 -2.2679424
H 1.2081462 -12.5401947 -3.5381929
C 3.1279736 -11.9299209 -3.3706337
H 3.7279360 -11.4201661 -2.6056435
C 3.8985958 -13.1821511 -3.8317212
H 3.2045756 -13.9120662 -4.2895438
H 4.6446384 -12.9083600 -4.5918828
C 4.5926935 -13.7141658 -2.6177426
N 3.9130962 -13.8275617 -1.4100055
C 4.8223496 -14.0849295 -0.4664342
H 4.6261972 -14.2355491 0.5929180
N 6.0604017 -14.1463371 -1.0105872
C 7.3100571 -14.3873992 -0.2850745
```

*To whom correspondence should be addressed

H 7.9710222 -13.5128431 -0.3950692
H 7.0758899 -14.5460490 0.7784749
H 7.8056983 -15.2830565 -0.6964442
C 5.9304940 -13.9237933 -2.3713437
H 6.7812014 -13.9295153 -3.0457323
C 2.7620395 -10.9335152 -4.4742889
O 1.8677970 -11.2401210 -5.2851186
N 3.3970727 -9.7647783 -4.3610543
H 4.1314678 -9.6663177 -3.6472305
C 3.2047868 -8.6566228 -5.2754040
H 3.7499058 -8.8811998 -6.2160600
H 2.1318171 -8.6063797 -5.5433467
H 3.5511220 -7.6984189 -4.8559565
H -4.4228467 -13.3699415 -1.8636026
C -3.5444771 -12.8198880 -2.2829300
H -3.7550834 -12.6050971 -3.3465505
H -3.4563048 -11.8642041 -1.7475947
C -2.2480717 -13.5555373 -2.1033464
N -1.9889377 -14.8854268 -2.4333816
H -2.6439287 -15.5801618 -2.8214710
C -0.6764117 -15.1493158 -2.1955498
H -0.2134313 -16.1191132 -2.3806093
N -0.0781229 -14.0643719 -1.7086161
C -1.0363755 -13.0701168 -1.6440515
H -0.8024426 -12.0631925 -1.2923141
H 1.4234414 -5.9841481 0.8697539
C 1.1474113 -6.5968487 -0.0477521
H 0.0985976 -6.3480266 -0.2977343
H 1.7839870 -6.2522172 -0.8834307
C 1.2983557 -8.1010116 0.1331168
C 0.3454855 -8.8675941 0.8394274
H -0.5197862 -8.3777014 1.2997666
C 0.4295764 -10.2660764 0.9193708
H -0.3466824 -10.8259484 1.4490290
C 1.5037350 -10.9398574 0.3172732
O 1.6451019 -12.3209588 0.3482282
H 1.1332106 -12.7663878 1.0897464
C 2.4640582 -10.1960049 -0.3868148
H 3.3158615 -10.7055239 -0.8451216
C 2.3460022 -8.8019347 -0.4952067

H 3.0868424 -8.2604564 -1.0940322
Cu 1.9214619 -13.8488162 -1.4020947
O 2.4264952 -16.2087231 -2.8848017
H 3.3661276 -16.3598174 -3.1741932
H 1.8695417 -16.6888577 -3.5493818
O 1.8560521 -15.6530266 -0.4270841
H 2.1193085 -16.1645092 -1.2706669
H 2.5876309 -15.8223979 0.2223756

62
Cu rest state (1) TPSS-D3/def2-TZVPD; Energ y = -3171.43914365641
N 1.8324466 -12.3373557 -2.6824422
H 1.4517910 -11.5367226 -2.1689483
H 1.1924336 -12.5027349 -3.4703195
C 3.1109828 -11.9221030 -3.3072604
H 3.7088011 -11.4229397 -2.5482558
C 3.8797659 -13.1631204 -3.7920675
H 3.1919162 -13.8768703 -4.2569163
H 4.6151746 -12.8782750 -4.5422411
C 4.5708407 -13.7069655 -2.5897563
N 3.8845831 -13.8428687 -1.3885759
C 4.7921217 -14.1007412 -0.4451272
H 4.5971210 -14.2729340 0.5983639
N 6.0259971 -14.1406763 -0.9852825
C 7.2745042 -14.3829728 -0.2576262
H 7.9428855 -13.5358268 -0.4030535
H 7.0438844 -14.4968032 0.7996261
H 7.7418368 -15.2930315 -0.6353330
C 5.9007938 -13.9022699 -2.3408861
H 6.7478433 -13.8867187 -3.0012755
C 2.7335783 -10.9261527 -4.3958566
O 1.8174777 -11.2353072 -5.1849274
N 3.3804702 -9.7715152 -4.3044761
H 4.1216414 -9.6887597 -3.6084892
C 3.1821739 -8.6552186 -5.2078698
H 3.6984221 -8.8842731 -6.1492451
H 2.1167527 -8.5959830 -5.4524256
H 3.5397849 -7.7122130 -4.7994223
H -4.4115477 -13.4202406 -1.8576020

C -3.5298457 -12.8863723 -2.2651870
H -3.7278479 -12.6750830 -3.3180825
H -3.4348200 -11.9428032 -1.7350808
C -2.2402838 -13.6271047 -2.0747593
N -1.9746034 -14.9548602 -2.4023264
H -2.6205902 -15.6559061 -2.7717990
C -0.6640027 -15.2102413 -2.1666118
H -0.2014138 -16.1671415 -2.3489107
N -0.0703144 -14.1230453 -1.6857673
C -1.0386164 -13.1352624 -1.6240432
H -0.8116526 -12.1361592 -1.2845273
H 1.4196020 -5.9053769 0.9033237
C 1.1417294 -6.5118846 -0.0058788
H 0.1054458 -6.2635473 -0.2511592
H 1.7731817 -6.1774304 -0.8323069
C 1.2855600 -8.0140251 0.1755153
C 0.3402002 -8.7725301 0.8840737
H -0.5113290 -8.2845081 1.3455951
C 0.4196911 -10.1637775 0.9632179
H -0.3464294 -10.7142412 1.4956716
C 1.4807684 -10.8358299 0.3556425
O 1.6279153 -12.2203035 0.3945516
H 1.1195877 -12.6548768 1.1230476
C 2.4307878 -10.1013723 -0.3559634
H 3.2707353 -10.6052489 -0.8184196
C 2.3191578 -8.7130299 -0.4582072
H 3.0480482 -8.1769360 -1.0568928
Cu 1.9152197 -13.8962450 -1.4073737
O 2.4797948 -16.3747144 -2.9947568
H 3.3941213 -16.5420302 -3.3080374
H 1.9018336 -16.8368215 -3.6320671
O 1.8902399 -15.7454698 -0.5052800
H 2.1693894 -16.2444192 -1.3286972
H 2.6075549 -15.9133161 0.1402913

62
Cu rest state (1) B3LYP-D3/def2-TZVPD; Energy = -3170.35495089520
N 1.8234746 -12.3680849 -2.7053875
H 1.4087166 -11.5644343 -2.2349587

H 1.2043436 -12.5775863 -3.4917734
C 3.0977993 -11.9368521 -3.3167479
H 3.6781574 -11.4276987 -2.5558952
C 3.8935888 -13.1601377 -3.7839340
H 3.2313922 -13.8824588 -4.2658601
H 4.6317288 -12.8616038 -4.5229521
C 4.5803384 -13.7039209 -2.5827502
N 3.8986673 -13.8536753 -1.3865000
C 4.8041015 -14.1141165 -0.4508695
H 4.6119145 -14.2937292 0.5896720
N 6.0314115 -14.1446885 -0.9889370
C 7.2769116 -14.3876677 -0.2726159
H 7.9392572 -13.5359139 -0.4009389
H 7.0574278 -14.5229168 0.7821083
H 7.7546348 -15.2839108 -0.6629191
C 5.9052103 -13.8985079 -2.3382237
H 6.7471909 -13.8728898 -3.0006672
C 2.7359193 -10.9483579 -4.4081344
O 1.8328392 -11.2589363 -5.1987259
N 3.3778818 -9.7979560 -4.3222248
H 4.1074071 -9.7043739 -3.6214325
C 3.1836697 -8.6880521 -5.2243104
H 3.7023026 -8.9093471 -6.1625815
H 2.1231145 -8.6188811 -5.4752433
H 3.5373125 -7.7452027 -4.8144256
H -4.4097318 -13.4249342 -1.8511046
C -3.5272382 -12.8939265 -2.2540128
H -3.7217190 -12.6842307 -3.3054196
H -3.4379947 -11.9502077 -1.7289709
C -2.2418922 -13.6322273 -2.0571928
N -1.9756011 -14.9529227 -2.3904517
H -2.6172636 -15.6479136 -2.7682172
C -0.6721308 -15.2087712 -2.1451511
H -0.2064807 -16.1617327 -2.3288996
N -0.0865295 -14.1312187 -1.6546129
C -1.0499694 -13.1445088 -1.5934430
H -0.8277856 -12.1496481 -1.2474813
H 1.4244622 -5.9062597 0.8997087
C 1.1492561 -6.5129236 -0.0086527
H 0.1178430 -6.2616782 -0.2589042

H 1.7812312 -6.1759923 -0.8296865
C 1.2907657 -8.0115876 0.1715992
C 0.3512792 -8.7642207 0.8847637
H -0.4953735 -8.2745762 1.3469410
C 0.4301581 -10.1509471 0.9667343
H -0.3321488 -10.6981209 1.5019631
C 1.4789524 -10.8258698 0.3523398
O 1.6084813 -12.2043201 0.3898805
H 1.1221771 -12.6362298 1.1285689
C 2.4230344 -10.0969255 -0.3621991
H 3.2522167 -10.6015832 -0.8342172
C 2.3157347 -8.7127414 -0.4634828
H 3.0410642 -8.1816046 -1.0654270
Cu 1.9201352 -13.8932447 -1.3863176
O 2.4054677 -16.3517470 -2.9653515
H 3.3213719 -16.5055427 -3.2704687
H 1.8414047 -16.8075971 -3.6148119
O 1.8907283 -15.7193701 -0.4180382
H 2.1277444 -16.2662146 -1.2071619
H 2.5963092 -15.8968140 0.2318445

62
Cu rest state reduced (2) TPSS-D3/def2-SV(P); Energy = -3169.55536959113
N 1.4328883 -12.7082474 -3.2515454
H 0.7319083 -12.0205958 -2.9336259
H 1.1515812 -12.9094947 -4.2297969
C 2.7261940 -11.9986101 -3.3844216
H 2.9549400 -11.5370357 -2.4139662
C 3.8459487 -13.0157944 -3.7181182
H 3.4380151 -13.7867688 -4.4009217
H 4.6588032 -12.5038450 -4.2562420
C 4.3952496 -13.6199268 -2.4626829
N 3.5685632 -14.1250680 -1.4665036
C 4.3453630 -14.4464923 -0.4343682
H 3.9868220 -14.8872121 0.4956464
N 5.6492993 -14.1735563 -0.7159515
C 6.8150436 -14.4349450 0.1260011
H 7.5929083 -13.6890057 -0.1084563
H 6.5337069 -14.3498068 1.1881248

H 7.2100204 -15.4481902 -0.0669104
C 5.6911457 -13.6626125 -2.0036772
H 6.6203006 -13.3562638 -2.4680673
C 2.5615578 -10.9198416 -4.4550707
O 1.7682172 -11.1427047 -5.3915425
N 3.2501428 -9.7871601 -4.2565705
H 3.9410981 -9.7487307 -3.4949339
C 3.2519002 -8.7047124 -5.2241434
H 3.9135541 -8.9854414 -6.0732957
H 2.2295784 -8.6363843 -5.6457011
H 3.5628254 -7.7224961 -4.8221127
H -4.5555026 -13.6975505 -1.6755748
C -3.6161627 -13.1936036 -2.0189069
H -3.7390308 -12.9646059 -3.0953705
H -3.5133900 -12.2344691 -1.4884326
C -2.3749449 -13.9917710 -1.7503977
N -2.1692212 -15.3378474 -2.0467158
H -2.8469211 -16.0053602 -2.4403218
C -0.8582510 -15.6371021 -1.8043312
H -0.4130811 -16.6223872 -1.9514143
N -0.2071466 -14.5522563 -1.3799650
C -1.1437551 -13.5347675 -1.3118451
H -0.8615170 -12.5251859 -1.0060139
H 1.3586912 -5.7593696 0.9371826
C 1.0253454 -6.3440132 0.0255141
H -0.0427671 -6.1065680 -0.1421606
H 1.5965481 -5.9638653 -0.8411434
C 1.2357409 -7.8397751 0.1549889
C 0.3665541 -8.6689405 0.8928506
H -0.4948764 -8.2352817 1.4153946
C 0.5378026 -10.0618870 0.9282435
H -0.1774408 -10.6889516 1.4715192
C 1.6064249 -10.6620027 0.2340041
O 1.8249109 -12.0109706 0.1888835
H 1.3243256 -12.5044672 0.9070817
C 2.4886551 -9.8397271 -0.4885468
H 3.3355785 -10.2880100 -1.0130155
C 2.2944581 -8.4576995 -0.5370363
H 2.9766328 -7.8540871 -1.1463688
Cu 1.6549335 -14.2350920 -1.8584410

O 2.0446641 -16.2925320 -2.7686810
H 3.0079258 -16.4153668 -2.9675865
H 1.5734948 -16.6330198 -3.5701773
O 1.6762460 -15.9390215 0.6340391
H 2.0740836 -16.7185720 0.1791626
H 1.6389558 -15.2448171 -0.0812378

62
Cu rest state reduced (2) TPSS-D3/def2-TZVPD; Energy = -3171.41970542255
N 1.4518795 -12.5569806 -2.9969150
H 0.8607263 -11.8274967 -2.5896404
H 1.0422381 -12.7242411 -3.9250836
C 2.7726429 -11.9500008 -3.2856179
H 3.1374917 -11.4840643 -2.3717127
C 3.7731071 -13.0516406 -3.6960948
H 3.2593557 -13.7876408 -4.3248501
H 4.5738377 -12.6124055 -4.2927782
C 4.3576620 -13.6663061 -2.4701628
N 3.5646664 -14.1310903 -1.4247010
C 4.3834155 -14.4374027 -0.4220919
H 4.0799152 -14.8472948 0.5269126
N 5.6699471 -14.1966834 -0.7712198
C 6.8679691 -14.4587173 0.0256963
H 7.6246017 -13.7172847 -0.2351302
H 6.6262530 -14.3792375 1.0856859
H 7.2484562 -15.4600022 -0.1878463
C 5.6634839 -13.7215611 -2.0696781
H 6.5709013 -13.4459098 -2.5731564
C 2.5638067 -10.9016727 -4.3638365
O 1.7223518 -11.1477620 -5.2550700
N 3.2500574 -9.7721754 -4.2148003
H 3.9654622 -9.7312474 -3.4875188
C 3.1819819 -8.6787669 -5.1650009
H 3.7657196 -8.9556661 -6.0552791
H 2.1416995 -8.5958663 -5.5010710
H 3.5281885 -7.7220326 -4.7742921
H -4.5747623 -13.7484169 -1.6633652
C -3.6406902 -13.2497299 -1.9974077
H -3.7611716 -13.0137305 -3.0591930

H -3.5312648 -12.3083662 -1.4607505
C -2.4013138 -14.0500459 -1.7412383
N -2.1649674 -15.3727630 -2.1039470
H -2.8318568 -16.0464690 -2.4862243
C -0.8469450 -15.6459971 -1.9067516
H -0.3915412 -16.6055572 -2.0972774
N -0.2166899 -14.5695401 -1.4438190
C -1.1793540 -13.5812843 -1.3154943
H -0.9215834 -12.5846469 -0.9885996
H 1.3568830 -5.6369782 0.9889980
C 1.0243375 -6.2080773 0.0763648
H -0.0303502 -5.9677253 -0.0893832
H 1.5980606 -5.8317480 -0.7739382
C 1.2295656 -7.7013632 0.2000385
C 0.3695917 -8.5288237 0.9351793
H -0.4844098 -8.1052159 1.4562099
C 0.5498539 -9.9129543 0.9756184
H -0.1527960 -10.5348601 1.5206410
C 1.6138802 -10.5008618 0.2819418
O 1.8648273 -11.8489014 0.2621185
H 1.3427628 -12.3508604 0.9421264
C 2.4756091 -9.6849037 -0.4548784
H 3.3083998 -10.1236831 -0.9893340
C 2.2774881 -8.3104105 -0.4985934
H 2.9415331 -7.7073426 -1.1104894
Cu 1.6578409 -14.1794392 -1.6988879
O 2.1370433 -16.2606540 -3.0642606
H 3.0776232 -16.4187776 -3.2909918
H 1.6326875 -16.6454516 -3.8079749
O 1.5269784 -16.1658296 0.5911254
H 1.9566883 -16.9961598 0.3109866
H 1.6589284 -15.5422320 -0.1688133

62
Cu rest state reduced (2) TPSS-D3/def2-TZVPD; Energy = -3170.34397636151
N 1.4708637 -12.4326396 -2.8815355
H 0.9456715 -11.6711615 -2.4585312
H 0.9935351 -12.6213425 -3.7633421
C 2.7982070 -11.9179739 -3.2598095

H 3.2340818 -11.4310086 -2.3941742
C 3.7349321 -13.0689797 -3.6682557
H 3.1754690 -13.8031181 -4.2518882
H 4.5222045 -12.6805681 -4.3106601
C 4.3540296 -13.6723701 -2.4563042
N 3.6027771 -14.1150043 -1.3796618
C 4.4514772 -14.4241666 -0.4141507
H 4.1831797 -14.8216650 0.5473403
N 5.7205025 -14.2062311 -0.8125122
C 6.9335608 -14.4729950 -0.0572214
H 7.6672095 -13.7017988 -0.2829337
H 6.7120015 -14.4586182 1.0069928
H 7.3419802 -15.4467468 -0.3256245
C 5.6702621 -13.7422949 -2.1091617
H 6.5563505 -13.4841573 -2.6524436
C 2.5964479 -10.9035107 -4.3655173
O 1.7749867 -11.1739569 -5.2548624
N 3.2653034 -9.7697069 -4.2289972
H 3.9656217 -9.7068853 -3.4963080
C 3.1856564 -8.6847460 -5.1767736
H 3.7610350 -8.9517956 -6.0707782
H 2.1476322 -8.5941613 -5.5062683
H 3.5307026 -7.7303593 -4.7852764
H -4.5758060 -13.7376462 -1.6635746
C -3.6470176 -13.2375324 -1.9960264
H -3.7634324 -13.0119425 -3.0572932
H -3.5507065 -12.2917264 -1.4713370
C -2.4051079 -14.0196428 -1.7242465
N -2.1387552 -15.3287045 -2.0981301
H -2.7837370 -16.0050419 -2.5004010
C -0.8285610 -15.5821493 -1.8636702
H -0.3473168 -16.5244720 -2.0634168
N -0.2390669 -14.5136736 -1.3611218
C -1.2104570 -13.5418764 -1.2536498
H -0.9776617 -12.5475600 -0.9122775
H 1.3576557 -5.6551697 0.9824832
C 1.0254330 -6.2272018 0.0752913
H -0.0254762 -5.9863125 -0.0909321
H 1.5945670 -5.8525749 -0.7742669
C 1.2259325 -7.7177255 0.2018967

C 0.3607101 -8.5346011 0.9333392
H -0.4913716 -8.1044462 1.4441411
C 0.5346669 -9.9146355 0.9854436
H -0.1693378 -10.5271767 1.5318353
C 1.5968619 -10.5105193 0.3066924
O 1.8391345 -11.8521401 0.3049413
H 1.3271570 -12.3503024 0.9850050
C 2.4628765 -9.7052672 -0.4273166
H 3.2946912 -10.1496269 -0.9502676
C 2.2719703 -8.3343070 -0.4831205
H 2.9414129 -7.7417936 -1.0930135
Cu 1.6655518 -14.0703809 -1.5564497
O 2.1274421 -16.3191042 -3.0521886
H 3.0660733 -16.4608818 -3.2693130
H 1.6361888 -16.7084277 -3.7936244
O 1.5312333 -16.1941692 0.6161967
H 1.9599465 -17.0251701 0.3576143
H 1.7124455 -15.5711483 -0.1129353

67
Cu-O2 equatorial (3eq, triplet) TPSS-D3/def2-SV(P); Energy = -3396.13661038825
N 1.7007705 -12.6433672 -2.8683847
H 1.1836240 -11.8938933 -2.3839948
H 1.1492279 -12.8485644 -3.7207687
C 2.9786489 -12.0763589 -3.3605922
H 3.4827434 -11.5848783 -2.5162722
C 3.8875948 -13.2282612 -3.8415739
H 3.2785008 -13.9765587 -4.3821671
H 4.6552776 -12.8383695 -4.5271160
C 4.5605421 -13.8167130 -2.6413828
N 3.8524187 -14.1444962 -1.4924969
C 4.7436810 -14.4521915 -0.5556645
H 4.4936948 -14.7891798 0.4496232
N 6.0069615 -14.3432953 -1.0443662
C 7.2420927 -14.5951785 -0.3084346
H 6.9882058 -14.8239505 0.7382713
H 7.7795591 -15.4520205 -0.7525853
H 7.8865751 -13.6999910 -0.3456226
C 5.9027305 -13.9534082 -2.3712017

H 6.7689334 -13.7924870 -3.0029562
C 2.6568600 -11.0404168 -4.4378752
O 1.8400103 -11.3384675 -5.3348510
N 3.2471761 -9.8486660 -4.2628594
H 3.9620344 -9.7585379 -3.5284265
C 3.1128871 -8.7479874 -5.2013115
H 3.6574709 -9.0120348 -6.1334774
H 2.0449455 -8.6634808 -5.4863709
H 3.4828094 -7.7788291 -4.8120308
H -4.5723344 -13.6773710 -1.7156372
C -3.6422834 -13.1605682 -2.0685760
H -3.8019560 -12.8980538 -3.1320039
H -3.5313544 -12.2184338 -1.5100575
C -2.3787376 -13.9452966 -1.8751598
N -2.1523539 -15.2750258 -2.2263006
H -2.8342998 -15.9556849 -2.5902978
C -0.8256926 -15.5436636 -2.0631299
H -0.3599457 -16.5072488 -2.2792422
N -0.1917021 -14.4649972 -1.6201062
C -1.1364797 -13.4722172 -1.4848548
H -0.8684039 -12.4682275 -1.1491315
H 1.3950420 -5.9061874 0.8936972
C 1.0829529 -6.5172181 -0.0137264
H 0.0285904 -6.2571839 -0.2293073
H 1.6946807 -6.1772155 -0.8697880
C 1.2318614 -8.0204125 0.1625667
C 0.3116770 -8.7837175 0.9114901
H -0.5341229 -8.2912715 1.4057471
C 0.4027490 -10.1823641 0.9927619
H -0.3533135 -10.7448761 1.5490218
C 1.4419991 -10.8663802 0.3337777
O 1.5887567 -12.2288342 0.3353298
H 1.0787942 -12.6896138 1.0638553
C 2.3671261 -10.1142866 -0.4134827
H 3.1808220 -10.6302743 -0.9280549
C 2.2539394 -8.7223464 -0.5067804
H 2.9714709 -8.1814148 -1.1344250
Cu 1.8597739 -14.3169076 -1.5680620
O 2.1484722 -15.9351211 -3.1560198
H 1.6097458 -16.4088625 -3.8518120

H 3.0763948 -16.2839830 -3.2639058
O 1.5978302 -15.5067202 0.0702032
O 2.4634644 -15.5289418 1.0109570
O 4.6922212 -17.0618950 -3.7556133
H 4.6975179 -18.0236447 -3.9908020
H 5.3219010 -16.6009761 -4.3667176
O 0.8900076 -17.4296478 -5.1437811
H 1.2970555 -16.9244916 -5.9090157
H 1.5105032 -18.2190472 -5.1021909

67
Cu-O2 equatorial (3eq, singlet) TPSS-D3/def2-SV(P); Energy = -3396.13133136967
N 1.7088648 -12.6449968 -2.8626468
H 1.1903767 -11.8951750 -2.3800318
H 1.1558736 -12.8575560 -3.7123056
C 2.9843968 -12.0769212 -3.3595311
H 3.4903538 -11.5838995 -2.5171022
C 3.8920182 -13.2289412 -3.8413914
H 3.2827134 -13.9757137 -4.3838457
H 4.6618467 -12.8389923 -4.5244036
C 4.5597575 -13.8185190 -2.6390754
N 3.8477233 -14.1415270 -1.4914140
C 4.7344360 -14.4495133 -0.5501007
H 4.4763551 -14.7848870 0.4536894
N 5.9992544 -14.3446247 -1.0354283
C 7.2322554 -14.5967996 -0.2959230
H 6.9761213 -14.8168505 0.7520689
H 7.7662957 -15.4592286 -0.7333086
H 7.8805569 -13.7046498 -0.3392377
C 5.9004996 -13.9578359 -2.3637262
H 6.7693678 -13.8001876 -2.9926575
C 2.6568342 -11.0415058 -4.4361497
O 1.8372479 -11.3407169 -5.3300430
N 3.2467841 -9.8493549 -4.2626058
H 3.9629786 -9.7587974 -3.5294793
C 3.1097394 -8.7482103 -5.2002675
H 3.6520632 -9.0120412 -6.1337293
H 2.0410906 -8.6637353 -5.4826237
H 3.4808418 -7.7792043 -4.8113483

H -4.5777281 -13.6712864 -1.7175846
C -3.6498401 -13.1524451 -2.0722913
H -3.8117058 -12.8910047 -3.1356231
H -3.5401676 -12.2097153 -1.5144793
C -2.3837375 -13.9331839 -1.8805962
N -2.1541319 -15.2638287 -2.2262399
H -2.8349083 -15.9482670 -2.5854451
C -0.8260286 -15.5271876 -2.0680123
H -0.3572291 -16.4899707 -2.2809204
N -0.1947597 -14.4437572 -1.6330095
C -1.1417383 -13.4535675 -1.4979860
H -0.8765445 -12.4470963 -1.1673756
H 1.3952849 -5.9062846 0.8946185
C 1.0835396 -6.5175403 -0.0127128
H 0.0291757 -6.2577171 -0.2285224
H 1.6953061 -6.1774219 -0.8686860
C 1.2324153 -8.0208749 0.1630204
C 0.3123986 -8.7847064 0.9118316
H -0.5326021 -8.2923760 1.4075497
C 0.4022401 -10.1835937 0.9904533
H -0.3536981 -10.7465787 1.5463477
C 1.4402058 -10.8674254 0.3291665
O 1.5844193 -12.2304023 0.3271156
H 1.0779348 -12.6920657 1.0583070
C 2.3658313 -10.1148098 -0.4167962
H 3.1795899 -10.6303579 -0.9318175
C 2.2536360 -8.7225584 -0.5078098
H 2.9713861 -8.1812646 -1.1348904
Cu 1.8554807 -14.3053392 -1.5564475
O 2.1389069 -15.9216504 -3.1610148
H 1.6025475 -16.4022337 -3.8540083
H 3.0644918 -16.2800796 -3.2564789
O 1.5770060 -15.4987914 0.0595792
O 2.4490604 -15.5235304 1.0044469
O 4.6784461 -17.0714768 -3.7368749
H 4.6830716 -18.0366313 -3.9611390
H 5.3053033 -16.6173425 -4.3548978
O 0.8877767 -17.4295845 -5.1431306
H 1.2956457 -16.9259014 -5.9089482
H 1.5080400 -18.2189032 -5.0991837

67
Cu-O2 axial (3ax, triplet) TPSS-D3/def2-SV(P); Energy = -3396.11491775603
N 1.6940975 -12.6065113 -2.8633083
H 1.1433963 -11.8724424 -2.3912019
H 1.1627909 -12.8442186 -3.7227335
C 2.9642751 -12.0059055 -3.3428779
H 3.4449897 -11.5050762 -2.4926902
C 3.9144503 -13.1128415 -3.8357588
H 3.3452455 -13.8703848 -4.4069523
H 4.6684192 -12.6785908 -4.5099061
C 4.6004313 -13.6947074 -2.6399849
N 3.9119219 -13.9340145 -1.4576591
C 4.8183611 -14.2843842 -0.5455871
H 4.6187964 -14.5622216 0.4881816
N 6.0655892 -14.2770140 -1.0816113
C 7.3130373 -14.5723320 -0.3818129
H 7.9977716 -13.7131638 -0.4733905
H 7.0866257 -14.7503389 0.6801217
H 7.7830222 -15.4703691 -0.8191733
C 5.9381326 -13.9176093 -2.4118843
H 6.7886781 -13.8398074 -3.0796141
C 2.6105148 -10.9675085 -4.4089352
O 1.7443589 -11.2463614 -5.2596437
N 3.2526410 -9.8001379 -4.2651050
H 3.9909794 -9.7274749 -3.5522497
C 3.1191919 -8.7006339 -5.2030646
H 3.6650849 -8.9639123 -6.1345399
H 2.0515764 -8.6172916 -5.4867402
H 3.4899073 -7.7368223 -4.8084877
H -4.5880530 -13.6353380 -1.7251188
C -3.6533466 -13.1272413 -2.0783920
H -3.7945290 -12.8923559 -3.1508462
H -3.5500183 -12.1720387 -1.5418968
C -2.3911869 -13.9033221 -1.8428769
N -2.1235701 -15.2153752 -2.2300753
H -2.7814160 -15.9039600 -2.6253846
C -0.8027703 -15.4714383 -2.0172289
H -0.3229865 -16.4139872 -2.2986043

N -0.2062076 -14.3988518 -1.4964007
C -1.1763799 -13.4267024 -1.3756615
H -0.9404838 -12.4263324 -1.0052743
H 1.4034838 -5.9465617 0.8785721
C 1.1012789 -6.5543855 -0.0331333
H 0.0467651 -6.3011655 -0.2557348
H 1.7169025 -6.2090998 -0.8841852
C 1.2581994 -8.0573834 0.1425126
C 0.3309961 -8.8304687 0.8732219
H -0.5260146 -8.3461375 1.3555877
C 0.4256032 -10.2300045 0.9434469
H -0.3399526 -10.7984553 1.4814311
C 1.4828540 -10.9006094 0.3023898
O 1.6343530 -12.2693742 0.2975456
H 1.1194223 -12.7307350 1.0198805
C 2.4219864 -10.1397806 -0.4143513
H 3.2557135 -10.6449766 -0.9057627
C 2.2981041 -8.7485657 -0.5087086
H 3.0230385 -8.2001534 -1.1208334
Cu 1.8899788 -14.1936669 -1.6214545
O 1.9570701 -15.5232190 -3.4813754
O 2.6195348 -16.6118015 -3.1664838
O 2.0067773 -16.0247207 -0.7524669
H 2.3502612 -16.5171439 -1.5954371
H 2.7171422 -16.1704336 -0.0767886
O 5.2015759 -16.8746941 -4.1290623
H 4.2143237 -16.8101716 -4.1500715
H 5.5599016 -16.0494176 -4.5410154
O 0.2951099 -17.7450436 -4.4717737
H 0.6637319 -16.8493840 -4.6308094
H 1.0808333 -18.3268346 -4.6823068

67
Cu-O2 axial (3ax, singlet) TPSS-D3/def2-SV(P); Energy = -3396.11317807983
N 1.7024507 -12.5829958 -2.8427256
H 1.1707988 -11.8401055 -2.3627180
H 1.1509227 -12.8233869 -3.6882976
C 2.9714341 -12.0042025 -3.3501267
H 3.4740380 -11.5037477 -2.5123374

C 3.8968941 -13.1282102 -3.8525051
H 3.3089461 -13.8827567 -4.4086343
H 4.6499105 -12.7093016 -4.5371024
C 4.5839807 -13.7077900 -2.6572744
N 3.8919664 -13.9392177 -1.4758240
C 4.7936757 -14.2805770 -0.5547894
H 4.5885178 -14.5490728 0.4802773
N 6.0418872 -14.2740989 -1.0858023
C 7.2871132 -14.5653191 -0.3790519
H 7.9729436 -13.7078451 -0.4760948
H 7.0571858 -14.7349926 0.6834589
H 7.7557096 -15.4679641 -0.8082360
C 5.9208458 -13.9254274 -2.4197765
H 6.7757101 -13.8494561 -3.0824062
C 2.6092493 -10.9661421 -4.4147146
O 1.7366200 -11.2443017 -5.2582528
N 3.2523825 -9.7992478 -4.2725881
H 3.9945226 -9.7274469 -3.5637311
C 3.1121403 -8.6970704 -5.2065219
H 3.6520275 -8.9582012 -6.1419246
H 2.0427791 -8.6125665 -5.4828957
H 3.4861151 -7.7350068 -4.8112176
H -4.5758120 -13.6329706 -1.7315994
C -3.6419431 -13.1242917 -2.0864616
H -3.7869488 -12.8870029 -3.1578455
H -3.5379260 -12.1701848 -1.5482170
C -2.3759659 -13.8975038 -1.8599154
N -2.1038488 -15.2075720 -2.2522761
H -2.7614164 -15.8995328 -2.6424881
C -0.7798795 -15.4570950 -2.0571310
H -0.2948226 -16.3944697 -2.3483943
N -0.1861961 -14.3802525 -1.5403916
C -1.1598643 -13.4134570 -1.4051970
H -0.9262752 -12.4127741 -1.0349207
H 1.4039423 -5.9506090 0.8786913
C 1.1053719 -6.5591395 -0.0340986
H 0.0518744 -6.3058991 -0.2608790
H 1.7243545 -6.2139277 -0.8827098
C 1.2607746 -8.0625593 0.1413929
C 0.3325400 -8.8336695 0.8730080

H -0.5230792 -8.3473715 1.3558990
C 0.4235392 -10.2332641 0.9434552
H -0.3427037 -10.7993698 1.4827058
C 1.4784504 -10.9064034 0.3015521
O 1.6270358 -12.2761939 0.2987845
H 1.1131255 -12.7354944 1.0235520
C 2.4174866 -10.1486160 -0.4182702
H 3.2488266 -10.6560209 -0.9113745
C 2.2973192 -8.7566823 -0.5122888
H 3.0226638 -8.2106496 -1.1259398
Cu 1.8839562 -14.1802743 -1.6113987
O 1.9503273 -15.5367051 -3.4683668
O 2.6353234 -16.6107314 -3.0957906
O 1.9953411 -15.9912486 -0.7324323
H 2.3523319 -16.4740941 -1.6007062
H 2.7103487 -16.1353843 -0.0620936
O 5.1784831 -16.8866702 -4.0964297
H 4.1877368 -16.8345089 -4.0687747
H 5.5054051 -16.0519758 -4.5112287
O 0.3167217 -17.7108721 -4.4697019
H 0.7163750 -16.8190351 -4.5794306
H 1.0932734 -18.3055261 -4.6778677

# 2 Molecular orbital plots

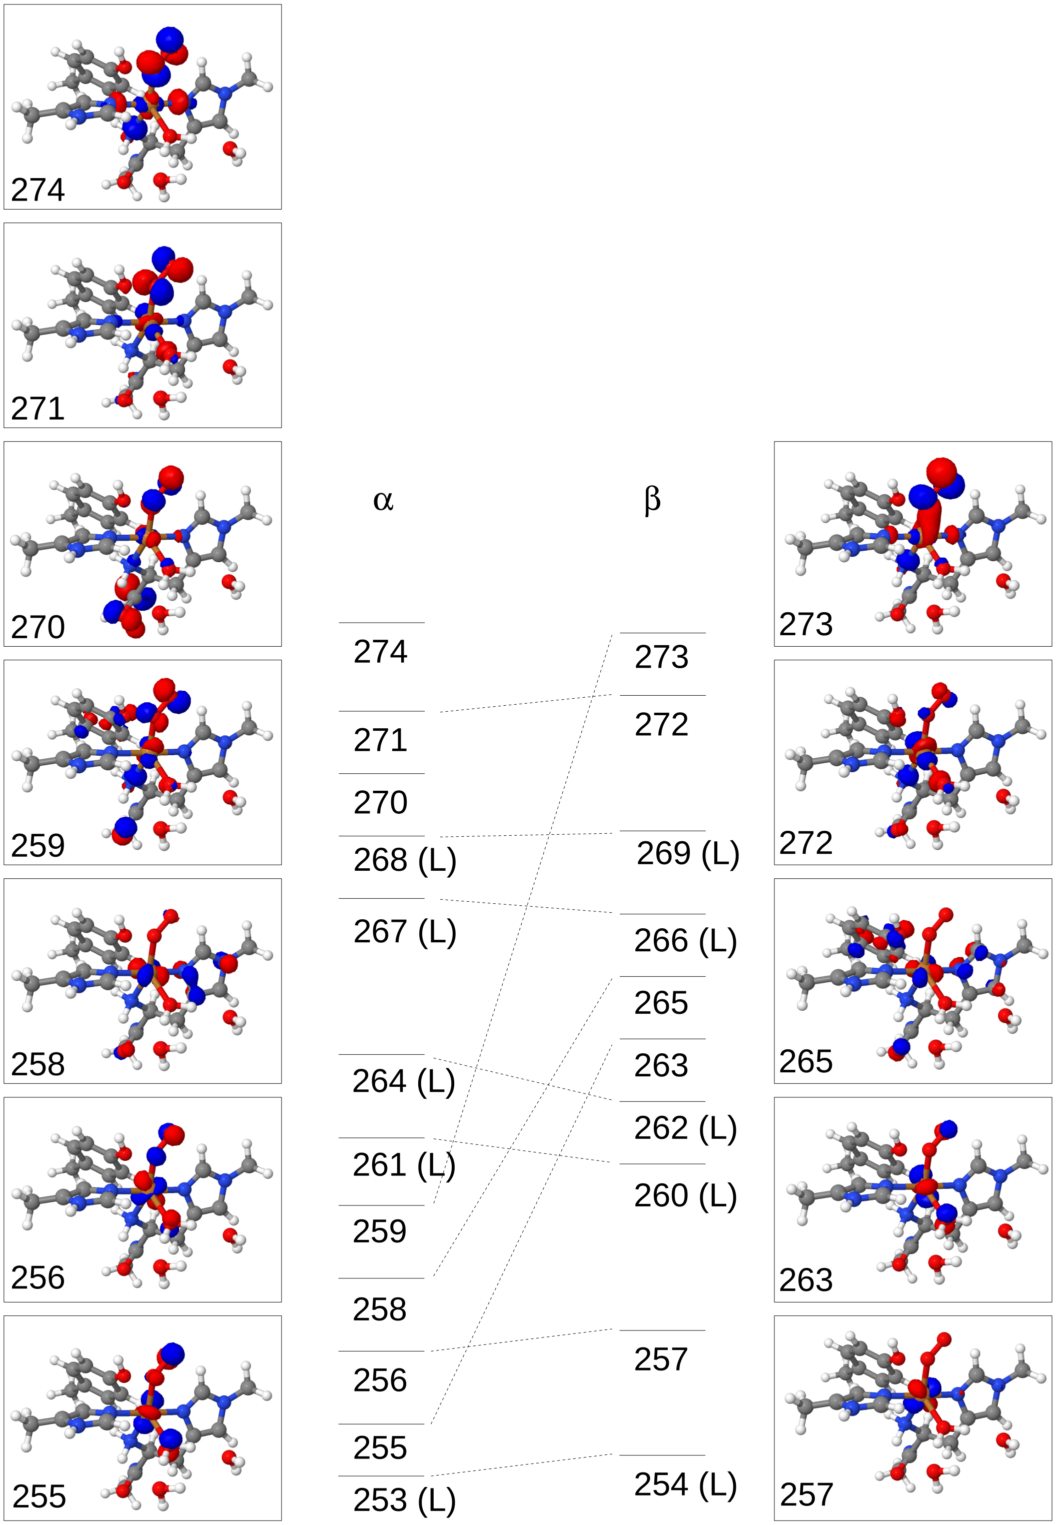


Figure S1: Selected molecular orbitals for $\mathbf{3}_{\mathrm{eq}}$. Orbitals marked with “(L)” are mainly centered on the ligands and are not shown.

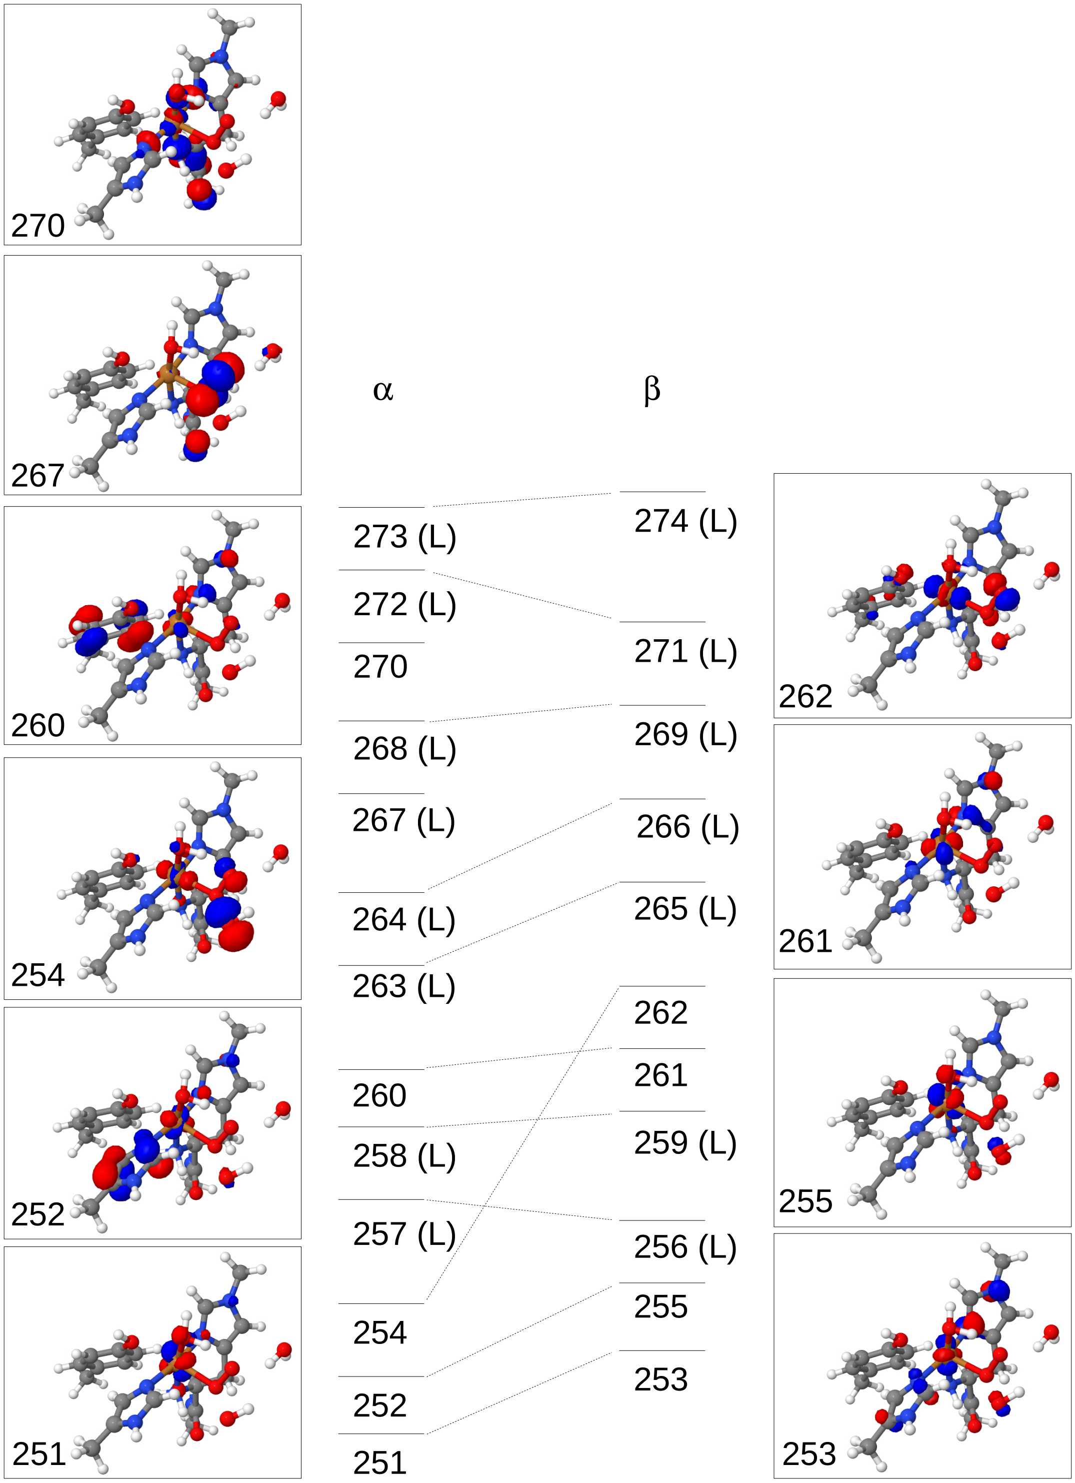


Figure S2: Selected molecular orbitals for $\mathbf{3}_{\mathrm{ax}}$. Orbitals marked with “(L)” are mainly centered on the ligands and are not shown.
